# Supplementary material for: Learning Approximately Optimal Contracts
Source: arXiv:1811.06736 source file (2022-07-13)
Supplement: Supplementary file 1 [file appendix.tex]

\end{document}
